# Supplementary material for: Constraints on Minute-Scale Transient Astrophysical Neutrino Sources
Source: arXiv:1807.11492 ancillary file (2019-02-27)
Supplement: Supplementary file 1 [file doublets_only_arxiv.pdf]

TABLE 1  
DOUBLETS DETECTED BETWEEN SEPTEMBER 2011 AND MAY 2016

| #  | MJD           | UTC times               | RA<br>(deg) | Dec<br>(deg) | 50% err<br>(deg) | 90% err<br>(deg) | angular sep.<br>(deg) | time diff.<br>(s) | $\lambda$ | <i>Swift</i> XRT obs. |
|----|---------------|-------------------------|-------------|--------------|------------------|------------------|-----------------------|-------------------|-----------|-----------------------|
| 1  | 55821.2041154 | 2011-09-17 04:53:55.566 | 299.05      | 22.15        | 0.4552           | 1.615            | 1.03                  | 81.690966         | -10.326   |                       |
| 2  | 55823.1214978 | 2011-09-19 02:54:57.408 | 244.18      | 18.41        | 0.4542           | 1.6042           | 2.7                   | 50.128059         | -4.631    |                       |
| 3  | 55825.3525364 | 2011-09-21 08:27:39.143 | 331.13      | 0.56         | 0.7236           | 2.4448           | 0.99                  | 21.151769         | -10.236   |                       |
| 4  | 55833.7743034 | 2011-09-29 18:34:59.817 | 346.77      | 35.34        | 0.6223           | 2.0396           | 1.56                  | 40.334708         | -9.187    |                       |
| 5  | 55848.5820038 | 2011-10-14 13:58:05.125 | 157.52      | 55.17        | 0.5014           | 1.725            | 2.47                  | 53.849557         | -7.645    |                       |
| 6  | 55849.934372  | 2011-10-15 22:25:29.739 | 205.05      | 13.44        | 1.0315           | 3.8409           | 3.33                  | 38.518204         | -4.42     |                       |
| 7  | 55851.5597246 | 2011-10-17 13:26:00.204 | 235.72      | 1.03         | 1.1405           | 3.7819           | 1.17                  | 33.729947         | -5.367    |                       |
| 8  | 55858.1119417 | 2011-10-24 02:41:11.760 | 225.08      | 59.81        | 0.1838           | 0.5991           | 1.29                  | 64.406847         | -11.223   | yes                   |
| 9  | 55866.9782735 | 2011-11-01 23:28:42.830 | 117.91      | 5.7          | 0.7586           | 2.5321           | 2.97                  | 60.869323         | -5.273    |                       |
| 10 | 55870.4101357 | 2011-11-05 09:50:35.727 | 28.52       | 1.19         | 1.67             | 7.354            | 3.01                  | 25.035609         | -2.693    |                       |
| 11 | 55887.0411986 | 2011-11-22 00:59:19.557 | 341.06      | 2.27         | 0.8082           | 2.647            | 0.46                  | 72.29811          | -5.861    |                       |
| 12 | 55890.2079319 | 2011-11-25 04:59:25.313 | 197.59      | 13.04        | 0.5946           | 1.9956           | 2.05                  | 57.666849         | -7.596    |                       |
| 13 | 55891.375548  | 2011-11-26 09:00:47.347 | 47.97       | 5.02         | 0.5781           | 2.0157           | 2.81                  | 59.376302         | -6.477    |                       |
| 14 | 55901.069622  | 2011-12-06 01:40:15.339 | 334.08      | 57.01        | 0.3654           | 1.2113           | 0.2                   | 99.131719         | -12.719   | yes                   |
| 15 | 55907.1674883 | 2011-12-12 04:01:10.986 | 291.69      | 3.47         | 0.5511           | 2.0245           | 2.92                  | 36.974874         | -7.015    |                       |
| 16 | 55911.2111554 | 2011-12-16 05:04:03.825 | 107.05      | 4.83         | 0.6366           | 2.0897           | 3.25                  | 75.637708         | -2.954    |                       |
| 17 | 55917.8707993 | 2011-12-22 20:53:57.057 | 276.22      | 10.29        | 0.2148           | 0.7837           | 1.54                  | 44.453401         | -10.687   |                       |
| 18 | 55919.7029319 | 2011-12-24 16:52:13.314 | 222.76      | 56.09        | 1.1658           | 3.8995           | 3.3                   | 33.919347         | -4.425    |                       |
| 19 | 55921.1906472 | 2011-12-26 04:34:31.917 | 19.59       | 9.66         | 0.4987           | 1.6958           | 1.72                  | 47.659106         | -9.337    |                       |
| 20 | 55923.1679512 | 2011-12-28 04:01:50.983 | 259.81      | 6.08         | 0.4119           | 1.3858           | 2.54                  | 6.179877          | -9.092    |                       |
| 21 | 55943.5648093 | 2012-01-17 13:33:19.521 | 26.78       | 14.44        | 0.4339           | 1.4908           | 1.54                  | 60.534181         | -8.737    |                       |
| 22 | 55943.9177553 | 2012-01-17 22:01:34.057 | 127.77      | 18.74        | 0.5727           | 1.8932           | 1.15                  | 5.855707          | -13.082   | yes                   |
| 23 | 55957.9707105 | 2012-01-31 23:17:49.391 | 160.66      | 3.24         | 0.7533           | 3.4869           | 2.52                  | 58.033842         | -5.931    |                       |
| 24 | 55959.3872712 | 2012-02-02 09:17:40.227 | 48.38       | 38.64        | 0.8867           | 3.0398           | 2.36                  | 61.608299         | -4.836    |                       |
| 25 | 55965.0100666 | 2012-02-08 00:14:29.753 | 21.53       | 10.22        | 0.244            | 0.8224           | 0.29                  | 79.520848         | -14.737   | yes                   |
| 26 | 55966.8781098 | 2012-02-09 21:04:28.685 | 268.22      | 13.5         | 0.4687           | 1.7228           | 3.1                   | 57.92012          | -1.5      |                       |
| 27 | 55970.1445427 | 2012-02-13 03:28:08.487 | 229.49      | 5.8          | 0.7021           | 2.2968           | 1.24                  | 42.854038         | -7.574    |                       |
| 28 | 55973.279478  | 2012-02-16 06:42:26.898 | 298.62      | 3.58         | 0.4386           | 1.4594           | 2.85                  | 8.84091           | -9.897    |                       |
| 29 | 55974.4333972 | 2012-02-17 10:24:05.520 | 101.81      | 10.75        | 0.4888           | 1.6329           | 2.07                  | 50.270791         | -8.533    |                       |
| 30 | 55989.6995592 | 2012-03-03 16:47:21.911 | 62.42       | 3.26         | 0.9346           | 3.3465           | 3.48                  | 1.192059          | -11.732   |                       |
| 31 | 55989.8321507 | 2012-03-03 19:58:17.819 | 341.92      | 3.21         | 1.1249           | 4.4918           | 3.49                  | 78.361306         | -2.655    |                       |
| 32 | 55990.7261891 | 2012-03-04 17:25:42.736 | 149.25      | 8.26         | 0.9453           | 3.151            | 3.21                  | 4.863307          | -9.055    |                       |
| 33 | 55991.3763453 | 2012-03-05 09:01:56.234 | 44.65       | 20.14        | 0.4494           | 1.4932           | 1.09                  | 92.062729         | -9.61     |                       |
| 34 | 55994.5223722 | 2012-03-08 12:32:12.955 | 107.11      | 5.61         | 0.403            | 1.343            | 1.68                  | 55.929744         | -8.998    |                       |
| 35 | 56001.6650356 | 2012-03-15 15:57:39.078 | 314.17      | 3.65         | 0.6643           | 2.1761           | 2.35                  | 32.938117         | -7.689    |                       |
| 36 | 56004.2420545 | 2012-03-18 05:48:33.510 | 301.17      | 35.87        | 0.4018           | 1.3487           | 2.23                  | 93.510285         | -6.445    |                       |
| 37 | 56004.3134984 | 2012-03-18 07:31:26.262 | 42.17       | 0.91         | 0.1967           | 0.6617           | 3.4                   | 86.294571         | 8.703     |                       |
| 38 | 56007.0120216 | 2012-03-21 00:17:18.664 | 162.38      | 5.75         | 0.6587           | 2.2114           | 2.49                  | 93.77579          | -5.553    |                       |
| 39 | 56007.1924041 | 2012-03-21 04:37:03.710 | 44.07       | 3.7          | 0.5979           | 1.9582           | 3.23                  | 50.459517         | -4.386    |                       |
| 40 | 56011.0637042 | 2012-03-25 01:31:44.044 | 256.68      | 3.13         | 0.1347           | 0.4459           | 2.1                   | 79.050207         | -0.66     |                       |
| 41 | 56012.6351204 | 2012-03-26 15:14:34.404 | 174.55      | 2.21         | 0.6402           | 2.2814           | 1.4                   | 94.848135         | -7.762    |                       |
| 42 | 56013.7738585 | 2012-03-27 18:34:21.372 | 200.89      | 15.11        | 0.6117           | 2.0132           | 1.46                  | 53.778922         | -8.619    |                       |
| 43 | 56014.3004914 | 2012-03-28 07:12:42.460 | 266.25      | 27.46        | 0.8389           | 2.8065           | 2.41                  | 13.234345         | -8.734    |                       |
| 44 | 56016.0465094 | 2012-03-30 01:06:58.414 | 104.48      | 17.22        | 0.3881           | 1.3919           | 1.32                  | 1.785199          | -17.612   | yes                   |
| 45 | 56028.2245152 | 2012-04-11 05:23:18.113 | 274.65      | 12.7         | 0.9485           | 4.1432           | 3.18                  | 76.491683         | -3.595    |                       |
| 46 | 56035.3806703 | 2012-04-18 09:08:09.917 | 240.57      | 0.01         | 0.441            | 1.4887           | 0.73                  | 65.077392         | -6.808    |                       |
| 47 | 56042.8159347 | 2012-04-25 19:34:56.758 | 11.69       | 2.91         | 0.2904           | 0.9894           | 2.1                   | 8.428633          | -13.107   |                       |
| 48 | 56053.6523807 | 2012-05-06 15:39:25.692 | 21.06       | 34.94        | 0.4937           | 1.6781           | 2.13                  | 4.93427           | -4.831    |                       |
| 49 | 56068.2222184 | 2012-05-21 05:19:59.670 | 101.2       | 20.48        | 1.4837           | 5.1526           | 1.34                  | 99.990768         | -0.848    |                       |
| 50 | 56070.9159925 | 2012-05-23 21:59:01.749 | 190.91      | 1.74         | 0.6389           | 2.2013           | 1.81                  | 46.443582         | -8.383    |                       |
| 51 | 56085.0707132 | 2012-06-07 01:41:49.617 | 332.66      | 15.93        | 0.6309           | 2.1682           | 2.83                  | 72.268325         | -4.606    |                       |
| 52 | 56087.0207949 | 2012-06-09 00:29:56.677 | 240.05      | 49.11        | 0.5031           | 1.7381           | 3.12                  | 9.263033          | -8.836    |                       |
| 53 | 56090.9496195 | 2012-06-12 22:47:27.128 | 221.65      | 3.72         | 0.4745           | 1.6416           | 2.5                   | 64.180108         | -6.598    |                       |
| 54 | 56094.3120531 | 2012-06-16 07:29:21.389 | 83.6        | 2.82         | 0.8448           | 2.9103           | 2.3                   | 26.195772         | -7.596    |                       |
| 55 | 56098.0389803 | 2012-06-20 00:56:07.898 | 198.99      | 3.83         | 0.7612           | 2.618            | 3.34                  | 12.200818         | -5.763    |                       |
| 56 | 56119.0348067 | 2012-07-11 00:50:07.300 | 134.15      | 0.57         | 0.4952           | 1.7061           | 2.81                  | 47.120033         | -5.593    |                       |
| 57 | 56120.1747145 | 2012-07-12 04:11:35.331 | 226.48      | 5.45         | 1.2304           | 4.2519           | 1.09                  | 56.039912         | -4.34     |                       |
| 58 | 56123.6783407 | 2012-07-15 16:16:48.638 | 280.5       | 27.93        | 1.8226           | 6.2752           | 3.41                  | 14.88714          | -1.791    |                       |
| 59 | 56126.8104771 | 2012-07-18 19:27:05.217 | 191.56      | 3.35         | 0.4953           | 1.7769           | 0.57                  | 59.769081         | -7.34     |                       |
| 60 | 56143.0006175 | 2012-08-04 00:00:53.351 | 339.29      | 6.46         | 0.6378           | 2.2005           | 3.3                   | 12.371287         | -6.627    |                       |
| 61 | 56143.0291628 | 2012-08-04 00:41:59.669 | 313.78      | 24.11        | 0.5695           | 1.9617           | 2.43                  | 40.618487         | -7.353    |                       |
| 62 | 56147.1288807 | 2012-08-08 03:05:35.295 | 238.77      | 9.0          | 0.3967           | 1.4415           | 0.98                  | 41.457755         | -9.411    | yes                   |
| 63 | 56153.6605654 | 2012-08-14 15:51:12.847 | 128.44      | 1.68         | 0.7754           | 2.67             | 3.49                  | 99.411547         | -3.078    |                       |
| 64 | 56162.4531487 | 2012-08-23 10:52:32.049 | 320.27      | 8.77         | 2.1436           | 7.3564           | 1.02                  | 66.862775         | 0.514     |                       |
| 65 | 56164.3244061 | 2012-08-25 07:47:08.685 | 13.76       | 39.81        | 0.4926           | 1.7007           | 3.18                  | 26.195444         | -6.583    |                       |
| 66 | 56165.0169678 | 2012-08-26 00:24:26.014 | 45.92       | 1.56         | 1.0414           | 3.6045           | 3.01                  | 65.24348          | -3.88     |                       |
| 67 | 56175.9168626 | 2012-09-05 22:00:16.928 | 67.17       | 32.41        | 1.0699           | 3.6879           | 2.08                  | 30.044394         | -6.279    |                       |
| 68 | 56180.1373293 | 2012-09-10 03:17:45.247 | 50.58       | 4.73         | 1.5914           | 5.4993           | 0.49                  | 42.261653         | -2.949    |                       |
| 69 | 56182.7032574 | 2012-09-12 16:52:41.436 | 48.7        | 16.2         | 0.4666           | 1.6097           | 2.9                   | 84.620913         | -5.377    |                       |
| 70 | 56183.0740213 | 2012-09-13 01:46:35.444 | 240.67      | 15.2         | 0.5265           | 1.8154           | 1.27                  | 72.102389         | -9.286    |                       |
| 71 | 56187.7555896 | 2012-09-17 18:08:02.943 | 60.65       | 5.21         | 0.5181           | 1.7829           | 1.85                  | 10.405754         | -11.695   | yes                   |
| 72 | 56190.9948777 | 2012-09-20 23:52:37.432 | 19.19       | 79.4         | 0.6764           | 2.3216           | 2.95                  | 56.005638         | -5.803    |                       |
| 73 | 56191.4213945 | 2012-09-21 10:06:48.482 | 296.63      | 1.27         | 0.8151           | 2.8411           | 0.94                  | 37.845354         | -8.08     |                       |
| 74 | 56200.517631  | 2012-09-30 12:25:23.322 | 97.67       | 0.82         | 1.3372           | 4.6224           | 1.54                  | 31.058944         | -5.103    |                       |
| 75 | 56215.1002318 | 2012-10-15 02:24:20.025 | 352.72      | 2.84         | 0.5014           | 1.7401           | 2.97                  | 55.920898         | -4.543    |                       |

TABLE 1 — *Continued*

| #   | MJD           | UTC times               | RA<br>(deg) | Dec<br>(deg) | 50% err<br>(deg) | 90% err<br>(deg) | angular sep.<br>(deg) | time diff.<br>(s) | $\lambda$ | <i>Swift</i> XRT obs. |
|-----|---------------|-------------------------|-------------|--------------|------------------|------------------|-----------------------|-------------------|-----------|-----------------------|
| 76  | 56220.0257715 | 2012-10-20 00:37:06.655 | 214.65      | 20.31        | 1.5114           | 5.3831           | 3.37                  | 91.053304         | -0.735    |                       |
| 77  | 56220.407984  | 2012-10-20 09:47:29.816 | 65.2        | 20.81        | 1.3792           | 4.7352           | 3.36                  | 6.474525          | -6.932    |                       |
| 78  | 56223.1987838 | 2012-10-23 04:46:14.918 | 339.95      | 6.55         | 0.434            | 1.4956           | 2.19                  | 3.702561          | -13.517   | yes                   |
| 79  | 56224.5469369 | 2012-10-24 13:07:35.350 | 327.84      | 5.32         | 0.5413           | 1.8575           | 2.3                   | 41.60016          | -8.204    |                       |
| 80  | 56234.4198734 | 2012-11-03 10:04:37.062 | 152.85      | 4.95         | 0.558            | 1.9603           | 1.82                  | 88.246962         | -7.209    |                       |
| 81  | 56242.1605218 | 2012-11-11 03:51:09.087 | 4.35        | 2.69         | 1.3378           | 4.5921           | 3.03                  | 61.126219         | -2.88     |                       |
| 82  | 56254.597623  | 2012-11-23 14:20:34.629 | 223.47      | 2.02         | 0.6185           | 2.1315           | 1.83                  | 60.499744         | -7.925    |                       |
| 83  | 56261.005995  | 2012-11-30 00:08:37.967 | 325.11      | 50.82        | 0.5724           | 1.9813           | 2.88                  | 45.821257         | -6.527    |                       |
| 84  | 56267.2621499 | 2012-12-06 06:17:29.755 | 99.66       | 61.14        | 0.4218           | 1.4535           | 3.33                  | 60.272175         | 2.343     |                       |
| 85  | 56271.5718589 | 2012-12-10 13:43:28.612 | 330.99      | 17.06        | 1.8259           | 6.2625           | 2.32                  | 40.078264         | -0.228    |                       |
| 86  | 56271.7043881 | 2012-12-10 16:54:19.133 | 59.95       | 21.72        | 0.4125           | 1.4258           | 2.68                  | 57.097806         | -6.401    |                       |
| 87  | 56271.855118  | 2012-12-10 20:31:22.197 | 50.83       | 6.56         | 0.8862           | 3.0501           | 3.31                  | 13.97144          | -6.849    |                       |
| 88  | 56274.2134875 | 2012-12-13 05:07:25.318 | 225.9       | 73.79        | 3.1274           | 10.8641          | 2.69                  | 77.015456         | 5.698     |                       |
| 89  | 56274.8317386 | 2012-12-13 19:57:42.210 | 120.2       | 8.38         | 0.8854           | 3.0459           | 3.04                  | 16.900259         | -6.375    |                       |
| 90  | 56275.7321108 | 2012-12-14 17:34:14.372 | 259.94      | 10.46        | 0.6926           | 2.4179           | 2.04                  | 41.191141         | -7.881    |                       |
| 91  | 56277.6660188 | 2012-12-16 15:59:04.025 | 259.73      | 0.36         | 1.2695           | 4.3808           | 3.44                  | 61.342139         | -2.745    |                       |
| 92  | 56282.095419  | 2012-12-21 02:17:24.199 | 213.96      | 7.76         | 0.2631           | 0.9107           | 0.85                  | 14.464866         | -14.765   | yes                   |
| 93  | 56286.6444524 | 2012-12-25 15:28:00.683 | 36.55       | 32.66        | 0.6737           | 2.3321           | 3.09                  | 33.195121         | -6.713    |                       |
| 94  | 56307.464426  | 2013-01-15 11:08:46.407 | 357.41      | 20.45        | 0.8234           | 2.8485           | 0.44                  | 0.81494           | -14.57    | yes                   |
| 95  | 56308.4334282 | 2013-01-16 10:24:08.197 | 85.89       | 8.57         | 1.7811           | 6.2081           | 2.93                  | 90.150267         | -0.003    |                       |
| 96  | 56309.2516373 | 2013-01-17 06:02:21.463 | 75.05       | 33.63        | 2.3069           | 7.9489           | 2.8                   | 43.002301         | 1.54      |                       |
| 97  | 56310.2182942 | 2013-01-18 05:14:20.617 | 33.28       | 75.95        | 0.6646           | 2.2851           | 2.48                  | 86.435388         | -5.281    |                       |
| 98  | 56310.9198136 | 2013-01-18 22:04:31.892 | 288.35      | 3.66         | 0.4962           | 1.7018           | 2.96                  | 47.328297         | -6.472    |                       |
| 99  | 56315.6356631 | 2013-01-23 15:15:21.287 | 138.75      | 11.85        | 1.0548           | 3.6404           | 2.52                  | 6.533165          | -8.857    |                       |
| 100 | 56316.5382586 | 2013-01-24 12:55:05.543 | 328.17      | 0.17         | 0.8131           | 2.7921           | 3.45                  | 42.85198          | -5.113    |                       |
| 101 | 56319.8652515 | 2013-01-27 20:45:57.726 | 92.31       | 1.96         | 0.9301           | 3.2109           | 2.15                  | 57.011807         | -5.645    |                       |
| 102 | 56321.4806844 | 2013-01-29 11:32:11.132 | 215.43      | 0.69         | 0.3067           | 1.0588           | 3.1                   | 93.443877         | 11.402    |                       |
| 103 | 56322.4024119 | 2013-01-30 09:39:28.390 | 238.54      | 2.6          | 0.6382           | 2.1959           | 0.41                  | 61.282615         | -8.267    |                       |
| 104 | 56334.0085683 | 2013-02-11 00:12:20.301 | 162.26      | 5.31         | 0.3695           | 1.2754           | 2.72                  | 96.877953         | -2.561    |                       |
| 105 | 56336.7831272 | 2013-02-13 18:47:42.187 | 164.36      | 35.79        | 0.467            | 1.6224           | 2.93                  | 5.520567          | -11.719   | yes                   |
| 106 | 56339.8810777 | 2013-02-16 21:08:45.117 | 339.36      | 13.44        | 0.9484           | 3.2229           | 1.43                  | 99.603079         | -5.284    |                       |
| 107 | 56345.6142604 | 2013-02-22 14:44:32.098 | 178.2       | 30.94        | 1.9495           | 6.8527           | 0.8                   | 42.587011         | -1.201    |                       |
| 108 | 56346.0984626 | 2013-02-23 02:21:47.167 | 40.85       | 0.95         | 0.5445           | 1.8684           | 2.85                  | 55.753029         | -4.385    |                       |
| 109 | 56346.8998803 | 2013-02-23 21:35:49.654 | 254.15      | 11.24        | 1.3852           | 4.7207           | 0.82                  | 56.879719         | -3.954    |                       |
| 110 | 56351.0986756 | 2013-02-28 02:22:05.572 | 330.22      | 12.81        | 0.7107           | 2.4315           | 2.1                   | 15.050944         | -9.692    |                       |
| 111 | 56353.3424694 | 2013-03-02 08:13:09.351 | 45.5        | 11.61        | 0.6511           | 2.2523           | 3.06                  | 74.344393         | -5.237    |                       |
| 112 | 56359.1214678 | 2013-03-08 02:54:54.819 | 224.4       | 47.17        | 0.8297           | 3.0326           | 3.32                  | 34.433929         | -5.583    |                       |
| 113 | 56359.9276591 | 2013-03-08 22:15:49.745 | 144.49      | 1.78         | 0.6982           | 2.4218           | 1.62                  | 6.088128          | -12.313   | yes                   |
| 114 | 56362.4051703 | 2013-03-11 09:43:26.716 | 172.44      | 21.37        | 0.3551           | 1.2366           | 1.84                  | 66.168185         | -8.892    |                       |
| 115 | 56375.9478787 | 2013-03-24 22:44:56.719 | 314.73      | 18.09        | 0.3716           | 1.2907           | 2.49                  | 92.111699         | -2.135    |                       |
| 116 | 56378.0896704 | 2013-03-27 02:09:07.520 | 338.54      | 25.7         | 0.6551           | 2.2169           | 1.42                  | 32.533096         | -6.379    |                       |
| 117 | 56378.6199836 | 2013-03-27 14:52:46.581 | 241.7       | 6.72         | 0.8129           | 2.794            | 2.91                  | 82.98925          | -4.271    |                       |
| 118 | 56378.8293093 | 2013-03-27 19:54:12.327 | 284.45      | 2.8          | 0.5467           | 1.9006           | 2.95                  | 7.562861          | -10.429   | yes                   |
| 119 | 56389.6234757 | 2013-04-07 14:57:48.299 | 208.95      | 8.83         | 0.7152           | 2.47             | 2.64                  | 68.44561          | -5.684    |                       |
| 120 | 56407.8753801 | 2013-04-25 21:00:32.842 | 64.17       | 3.88         | 0.2924           | 1.0199           | 2.6                   | 64.827949         | -8.275    |                       |
| 121 | 56409.1661453 | 2013-04-27 03:59:14.951 | 312.99      | 18.6         | 0.5903           | 2.0367           | 0.86                  | 81.568909         | -9.011    |                       |
| 122 | 56414.4767752 | 2013-05-02 11:26:33.374 | 90.17       | 3.76         | 0.3373           | 1.197            | 1.9                   | 61.887325         | -7.084    |                       |
| 123 | 56416.0932823 | 2013-05-04 02:14:19.592 | 20.36       | 21.33        | 1.2182           | 4.1892           | 2.87                  | 87.017796         | -1.609    |                       |
| 124 | 56429.6646215 | 2013-05-17 15:57:03.294 | 191.69      | 15.06        | 0.7208           | 2.4729           | 1.59                  | 1.103025          | -15.113   | yes                   |
| 125 | 56444.8365432 | 2013-06-01 20:04:37.328 | 16.93       | 14.05        | 0.8305           | 2.8772           | 1.48                  | 51.038729         | -7.01     |                       |
| 126 | 56453.6433481 | 2013-06-10 15:26:25.271 | 108.13      | 16.78        | 1.8467           | 6.3606           | 2.88                  | 8.453353          | -4.892    |                       |
| 127 | 56454.8114285 | 2013-06-11 19:28:27.426 | 148.48      | 5.97         | 0.8667           | 2.9806           | 1.27                  | 52.096242         | -7.308    |                       |
| 128 | 56463.1117325 | 2013-06-20 02:40:53.689 | 166.13      | 16.09        | 0.9147           | 3.1376           | 2.26                  | 98.367382         | -3.12     |                       |
| 129 | 56484.3780706 | 2013-07-11 09:04:25.303 | 82.86       | 19.98        | 0.5547           | 1.9205           | 3.47                  | 32.680178         | -6.399    |                       |
| 130 | 56497.4369206 | 2013-07-24 10:29:09.942 | 226.61      | 27.29        | 0.6427           | 2.217            | 1.27                  | 85.157082         | -7.692    |                       |
| 131 | 56500.1588114 | 2013-07-27 03:48:41.304 | 189.4       | 17.24        | 0.3893           | 1.3423           | 2.38                  | 71.740656         | -6.297    |                       |
| 132 | 56503.5172487 | 2013-07-30 12:24:50.284 | 40.27       | 56.03        | 1.2589           | 4.3698           | 3.22                  | 92.202304         | -1.364    |                       |
| 133 | 56513.0112915 | 2013-08-09 00:16:15.589 | 79.36       | 9.38         | 0.4905           | 1.7012           | 0.83                  | 51.837558         | -11.06    |                       |
| 134 | 56515.0210662 | 2013-08-11 00:30:20.122 | 303.91      | 19.37        | 1.0062           | 3.4669           | 0.58                  | 40.261212         | -6.511    |                       |
| 135 | 56516.3366163 | 2013-08-12 08:04:43.650 | 354.72      | 32.69        | 0.8591           | 2.9677           | 2.79                  | 4.681435          | -10.2     |                       |
| 136 | 56519.6519261 | 2013-08-15 15:38:46.417 | 299.36      | 4.26         | 0.4906           | 1.698            | 2.86                  | 92.325354         | -5.094    |                       |
| 137 | 56523.9260712 | 2013-08-19 22:13:32.553 | 314.88      | 56.68        | 0.6763           | 2.3231           | 2.31                  | 23.763388         | -8.408    |                       |
| 138 | 56528.1586367 | 2013-08-24 03:48:26.211 | 49.27       | 65.12        | 0.8015           | 2.7759           | 2.25                  | 52.771321         | -6.46     |                       |
| 139 | 56531.4010478 | 2013-08-27 09:37:30.526 | 242.94      | 3.55         | 0.4451           | 1.5315           | 2.9                   | 72.168763         | -2.93     |                       |
| 140 | 56536.0149683 | 2013-09-01 00:21:33.261 | 219.9       | 30.15        | 0.4934           | 1.6956           | 2.03                  | 93.000208         | -6.795    |                       |
| 141 | 56538.3165348 | 2013-09-03 07:35:48.606 | 155.42      | 9.25         | 0.9685           | 3.3464           | 2.89                  | 39.402227         | -5.349    |                       |
| 142 | 56538.3713042 | 2013-09-03 08:54:40.685 | 160.8       | 6.05         | 0.7771           | 2.6844           | 2.81                  | 25.691226         | -6.887    |                       |
| 143 | 56547.2663499 | 2013-09-12 06:23:32.634 | 154.88      | 59.56        | 1.9245           | 6.7176           | 3.17                  | 49.866905         | -0.932    |                       |
| 144 | 56559.1406597 | 2013-09-24 03:22:32.998 | 82.42       | 5.64         | 0.5598           | 1.9369           | 1.36                  | 37.917379         | -10.306   |                       |
| 145 | 56559.3280073 | 2013-09-24 07:52:19.834 | 222.49      | 37.22        | 0.7869           | 2.7222           | 2.14                  | 79.733909         | -5.901    |                       |
| 146 | 56566.4808973 | 2013-10-01 11:32:29.529 | 201.11      | 9.62         | 0.6814           | 2.3544           | 3.0                   | 66.10654          | -5.343    |                       |
| 147 | 56578.3396476 | 2013-10-13 08:09:05.553 | 203.92      | 6.96         | 0.4973           | 1.7088           | 2.85                  | 45.198905         | -7.419    |                       |
| 148 | 56583.5721865 | 2013-10-18 13:43:56.912 | 163.37      | 11.13        | 0.5614           | 1.9297           | 2.23                  | 31.394597         | -8.312    |                       |
| 149 | 56584.8104427 | 2013-10-19 19:27:02.245 | 352.15      | 29.03        | 0.8479           | 2.913            | 2.88                  | 67.401363         | -4.778    |                       |
| 150 | 56584.8439632 | 2013-10-19 20:15:18.416 | 33.52       | 6.17         | 0.3982           | 1.3783           | 1.65                  | 38.387707         | -10.003   |                       |
| 151 | 56586.0628037 | 2013-10-21 01:30:26.239 | 272.58      | 17.32        | 0.4469           | 1.54             | 2.73                  | 88.351431         | -3.687    |                       |

TABLE 1 — *Continued*

| #   | MJD           | UTC times               | RA<br>(deg) | Dec<br>(deg) | 50% err<br>(deg) | 90% err<br>(deg) | angular sep.<br>(deg) | time diff.<br>(s) | $\lambda$ | <i>Swift</i> XRT obs. |
|-----|---------------|-------------------------|-------------|--------------|------------------|------------------|-----------------------|-------------------|-----------|-----------------------|
| 152 | 56588.6687608 | 2013-10-23 16:03:00.933 | 21.14       | 2.0          | 0.6181           | 2.1344           | 3.34                  | 34.652311         | -3.936    |                       |
| 153 | 56591.2275926 | 2013-10-26 05:27:44.004 | 234.59      | 9.77         | 0.8288           | 2.8653           | 2.38                  | 20.688577         | -7.505    |                       |
| 154 | 56594.5662973 | 2013-10-29 13:35:28.086 | 195.25      | 32.72        | 1.4488           | 5.0637           | 1.75                  | 10.563673         | -5.316    |                       |
| 155 | 56595.0399223 | 2013-10-30 00:57:29.285 | 244.57      | 15.17        | 1.215            | 4.1954           | 3.47                  | 74.818894         | -2.409    |                       |
| 156 | 56600.9443039 | 2013-11-04 22:39:47.857 | 230.32      | 4.97         | 0.7645           | 2.6494           | 2.48                  | 49.499471         | -6.327    |                       |
| 157 | 56613.9128153 | 2013-11-17 21:54:27.238 | 306.21      | 8.0          | 0.6625           | 2.3034           | 3.34                  | 94.153217         | -2.558    |                       |
| 158 | 56617.3249171 | 2013-11-21 07:47:52.840 | 342.49      | 8.35         | 0.6839           | 2.3531           | 2.36                  | 23.08695          | -8.208    |                       |
| 159 | 56618.2982273 | 2013-11-22 07:09:26.834 | 10.49       | 10.99        | 0.8321           | 2.8687           | 2.19                  | 79.380674         | -5.606    |                       |
| 160 | 56630.1367038 | 2013-12-04 03:16:51.208 | 236.36      | 28.41        | 0.8171           | 2.8165           | 2.71                  | 68.355524         | -5.055    |                       |
| 161 | 56635.4490565 | 2013-12-09 10:46:38.480 | 146.42      | 20.93        | 0.3539           | 1.226            | 3.28                  | 78.672636         | -6.094    |                       |
| 162 | 56635.7300458 | 2013-12-09 17:31:15.958 | 275.15      | 50.76        | 0.4029           | 1.396            | 0.91                  | 72.260952         | -10.253   |                       |
| 163 | 56639.4289467 | 2013-12-13 10:17:40.996 | 208.89      | 32.54        | 0.664            | 2.2862           | 1.77                  | 64.176073         | -7.676    |                       |
| 164 | 56640.9178045 | 2013-12-14 22:01:38.309 | 215.18      | 3.88         | 0.3042           | 1.0563           | 2.79                  | 43.314501         | -2.415    |                       |
| 165 | 56644.1465848 | 2013-12-18 03:31:04.925 | 348.35      | 4.64         | 0.8716           | 3.0119           | 1.64                  | 97.599916         | -4.47     |                       |
| 166 | 56645.5014855 | 2013-12-19 12:02:08.345 | 185.44      | 3.48         | 1.122            | 3.945            | 3.35                  | 28.287271         | -4.859    |                       |
| 167 | 56647.8508394 | 2013-12-21 20:25:12.520 | 206.83      | 23.69        | 0.4048           | 1.3979           | 3.07                  | 45.338242         | -1.313    |                       |
| 168 | 56650.3899784 | 2013-12-24 09:21:34.136 | 302.96      | 9.29         | 0.7277           | 2.5053           | 2.89                  | 34.385344         | -6.372    |                       |
| 169 | 56662.7490844 | 2014-01-05 17:58:40.889 | 303.18      | 11.0         | 0.5413           | 1.8726           | 2.63                  | 47.297401         | -6.846    |                       |
| 170 | 56665.2285684 | 2014-01-08 05:29:08.312 | 121.04      | 12.78        | 0.484            | 1.6781           | 1.21                  | 6.311976          | -14.696   | yes                   |
| 171 | 56665.3660853 | 2014-01-08 08:47:09.772 | 77.86       | 0.3          | 1.0221           | 3.5294           | 3.09                  | 57.41305          | -3.97     |                       |
| 172 | 56673.3273347 | 2014-01-16 07:51:21.720 | 175.55      | 1.29         | 1.315            | 4.5529           | 1.15                  | 30.61027          | -4.655    |                       |
| 173 | 56674.1681804 | 2014-01-17 04:02:10.787 | 299.41      | 45.67        | 0.3909           | 1.3511           | 1.91                  | 8.425277          | -12.709   | yes                   |
| 174 | 56677.3508814 | 2014-01-20 08:25:16.151 | 194.61      | 16.9         | 0.3494           | 1.2101           | 3.46                  | 88.910605         | -2.987    |                       |
| 175 | 56677.902598  | 2014-01-20 21:39:44.465 | 92.38       | 4.36         | 0.5809           | 2.0024           | 1.54                  | 48.967889         | -7.008    |                       |
| 176 | 56686.8832042 | 2014-01-29 21:11:48.839 | 15.34       | 9.45         | 0.9358           | 3.2414           | 2.4                   | 15.078198         | -8.074    |                       |
| 177 | 56687.6750208 | 2014-01-30 16:12:01.795 | 77.33       | 4.51         | 0.8189           | 2.8231           | 2.9                   | 61.662299         | -4.865    |                       |
| 178 | 56688.3128019 | 2014-01-31 07:30:26.082 | 38.39       | 32.04        | 0.679            | 2.3564           | 2.04                  | 28.735561         | -8.658    |                       |
| 179 | 56705.6049692 | 2014-02-17 14:31:09.341 | 55.66       | 18.74        | 0.4738           | 1.645            | 1.17                  | 70.040397         | -9.794    |                       |
| 180 | 56709.1523853 | 2014-02-21 03:39:26.090 | 302.03      | 11.02        | 0.4181           | 1.445            | 3.06                  | 78.244822         | -6.35     |                       |
| 181 | 56710.5906984 | 2014-02-22 14:10:36.345 | 355.48      | 5.68         | 0.8505           | 2.9168           | 0.87                  | 2.107711          | -12.947   |                       |
| 182 | 56710.8743833 | 2014-02-22 20:59:06.714 | 174.76      | 14.54        | 0.3643           | 1.251            | 2.72                  | 37.511444         | -8.858    |                       |
| 183 | 56712.6575457 | 2014-02-24 15:46:51.946 | 159.22      | 7.71         | 0.5047           | 1.7707           | 1.47                  | 50.047133         | -9.852    |                       |
| 184 | 56714.794618  | 2014-02-26 19:04:14.995 | 155.37      | 16.91        | 0.2971           | 1.1882           | 2.06                  | 8.258182          | -12.868   | yes                   |
| 185 | 56717.4848594 | 2014-03-01 11:38:11.850 | 207.61      | 11.83        | 0.8135           | 2.8129           | 1.5                   | 87.282838         | -6.439    |                       |
| 186 | 56722.4499553 | 2014-03-06 10:47:56.133 | 150.45      | 16.78        | 0.417            | 1.4363           | 3.43                  | 4.238378          | -2.461    |                       |
| 187 | 56729.4487039 | 2014-03-13 10:46:08.019 | 101.28      | 30.68        | 1.4611           | 5.0251           | 3.0                   | 98.576085         | -1.424    |                       |
| 188 | 56731.0087521 | 2014-03-15 00:12:36.180 | 86.71       | 11.8         | 1.7129           | 5.8785           | 3.26                  | 46.01031          | -1.885    |                       |
| 189 | 56744.9123786 | 2014-03-28 21:53:49.512 | 39.76       | 18.65        | 0.4262           | 1.4656           | 1.54                  | 1.453982          | -17.178   |                       |
| 190 | 56749.2864289 | 2014-04-02 06:52:27.452 | 103.62      | 8.47         | 0.4196           | 1.45             | 1.66                  | 96.353154         | -5.596    |                       |
| 191 | 56766.0437154 | 2014-04-19 01:02:57.009 | 19.08       | 13.15        | 0.4297           | 1.4825           | 1.44                  | 75.570972         | -9.467    |                       |
| 192 | 56776.8921181 | 2014-04-29 21:24:39.004 | 96.87       | 19.53        | 0.4371           | 1.4993           | 1.62                  | 62.785612         | -9.434    |                       |
| 193 | 56782.6962356 | 2014-05-05 16:42:34.759 | 327.21      | 32.99        | 1.1055           | 3.8008           | 0.48                  | 24.44361          | -5.793    |                       |
| 194 | 56790.0224834 | 2014-05-13 00:32:22.566 | 349.16      | 8.38         | 0.4957           | 1.7004           | 3.32                  | 77.115881         | -5.425    |                       |
| 195 | 56790.0787253 | 2014-05-13 01:53:21.862 | 110.33      | 2.36         | 0.8829           | 3.0672           | 3.22                  | 73.028772         | -3.942    |                       |
| 196 | 56794.6516592 | 2014-05-17 15:38:23.354 | 117.3       | 45.43        | 0.3754           | 1.3073           | 2.48                  | 69.171307         | -4.667    |                       |
| 197 | 56797.8775569 | 2014-05-20 21:03:40.912 | 8.62        | 33.37        | 0.5934           | 2.0562           | 1.84                  | 47.780774         | -8.528    |                       |
| 198 | 56802.9303961 | 2014-05-25 22:19:46.224 | 68.74       | 14.73        | 1.1638           | 4.0009           | 1.26                  | 73.095057         | -4.357    |                       |
| 199 | 56803.0433474 | 2014-05-26 01:02:25.212 | 44.07       | 14.42        | 1.2711           | 4.385            | 1.98                  | 45.454479         | -4.553    |                       |
| 200 | 56804.2638889 | 2014-05-27 06:20:00.005 | 59.59       | 21.25        | 0.6242           | 2.1426           | 2.22                  | 39.67851          | -7.6      |                       |
| 201 | 56808.3154274 | 2014-05-31 07:34:12.923 | 64.72       | 2.23         | 1.2009           | 4.1547           | 2.23                  | 27.932906         | -5.722    |                       |
| 202 | 56810.5972434 | 2014-06-02 14:20:01.828 | 100.92      | 17.96        | 0.4914           | 1.6981           | 3.04                  | 41.88054          | -7.152    |                       |
| 203 | 56814.2474127 | 2014-06-06 05:56:16.460 | 142.13      | 38.49        | 0.8891           | 3.0637           | 2.18                  | 53.954907         | -5.011    |                       |
| 204 | 56824.3839078 | 2014-06-16 09:12:49.636 | 289.24      | 15.08        | 0.577            | 1.9915           | 2.38                  | 61.21104          | -6.365    |                       |
| 205 | 56832.6610349 | 2014-06-24 15:51:53.418 | 347.21      | 2.88         | 0.5131           | 1.7729           | 0.7                   | 70.024045         | -9.618    |                       |
| 206 | 56837.7537229 | 2014-06-29 18:05:21.658 | 118.19      | 11.95        | 0.9424           | 3.2585           | 0.78                  | 55.135395         | -6.031    |                       |
| 207 | 56838.2220117 | 2014-06-30 05:19:41.814 | 40.11       | 22.88        | 0.5945           | 2.049            | 0.7                   | 66.915332         | -9.422    |                       |
| 208 | 56840.2421031 | 2014-07-02 05:48:37.711 | 67.96       | 9.47         | 0.8042           | 2.7608           | 3.29                  | 23.629406         | -6.341    |                       |
| 209 | 56842.6783879 | 2014-07-04 16:16:52.718 | 298.07      | 12.21        | 1.4699           | 5.0915           | 0.85                  | 65.466359         | -2.924    |                       |
| 210 | 56847.6594567 | 2014-07-09 15:49:37.056 | 342.3       | 4.87         | 0.4149           | 1.469            | 1.96                  | 92.989591         | -6.503    |                       |
| 211 | 56850.3474441 | 2014-07-12 08:20:19.167 | 350.67      | 47.8         | 0.662            | 2.2714           | 3.22                  | 95.270735         | -4.201    |                       |
| 212 | 56857.4102607 | 2014-07-19 09:50:46.525 | 90.24       | 10.49        | 0.5636           | 1.9483           | 2.82                  | 3.621146          | -11.365   |                       |
| 213 | 56858.4535925 | 2014-07-20 10:53:10.390 | 89.55       | 27.12        | 0.3979           | 1.3734           | 1.24                  | 15.967322         | -13.512   |                       |
| 214 | 56866.4349065 | 2014-07-28 10:26:15.921 | 230.19      | 8.25         | 0.2753           | 0.9534           | 3.1                   | 39.502264         | -3.91     |                       |
| 215 | 56868.1217005 | 2014-07-30 02:55:14.922 | 74.16       | 1.85         | 0.7018           | 2.4106           | 2.71                  | 35.437116         | -6.979    |                       |
| 216 | 56881.8521264 | 2014-08-12 20:27:03.718 | 250.4       | 26.56        | 0.2409           | 0.8337           | 2.39                  | 59.580202         | -4.94     |                       |
| 217 | 56882.8180941 | 2014-08-13 19:38:03.329 | 19.02       | 84.76        | 9.047            | 31.456           | 1.57                  | 20.951692         | 10.299    |                       |
| 218 | 56883.7559784 | 2014-08-14 18:08:36.531 | 152.31      | 19.16        | 0.5981           | 2.0531           | 2.95                  | 97.086657         | -5.187    |                       |
| 219 | 56885.1268641 | 2014-08-16 03:02:41.055 | 342.54      | 36.79        | 0.7142           | 2.4721           | 0.89                  | 64.392971         | -8.533    |                       |
| 220 | 56887.6315768 | 2014-08-18 15:09:28.233 | 138.25      | 4.31         | 0.4237           | 1.4634           | 2.4                   | 39.431206         | -6.962    |                       |
| 221 | 56888.3178374 | 2014-08-19 07:37:41.150 | 129.98      | 5.01         | 0.2704           | 0.9289           | 2.52                  | 64.505823         | -3.017    |                       |
| 222 | 56892.4641173 | 2014-08-23 11:08:19.738 | 352.64      | 1.04         | 0.4323           | 1.5129           | 1.2                   | 70.365084         | -10.452   |                       |
| 223 | 56898.5797395 | 2014-08-29 13:54:49.496 | 267.3       | 4.56         | 0.36             | 1.259            | 1.59                  | 7.752738          | -14.214   | yes                   |
| 224 | 56898.6588094 | 2014-08-29 15:48:41.130 | 125.42      | 8.59         | 0.7195           | 2.4869           | 2.9                   | 91.159883         | -4.202    |                       |
| 225 | 56904.1909251 | 2014-09-04 04:34:55.929 | 323.69      | 67.6         | 0.7918           | 2.7355           | 3.2                   | 15.230288         | -7.23     |                       |
| 226 | 56910.4432676 | 2014-09-10 10:38:18.318 | 195.0       | 28.7         | 0.3843           | 1.3196           | 2.04                  | 71.922046         | -6.741    |                       |
| 227 | 56914.5407    | 2014-09-14 12:58:36.478 | 304.98      | 29.93        | 0.4522           | 1.5687           | 2.75                  | 3.396376          | -9.211    | yes                   |

TABLE 1 — *Continued*

| #   | MJD           | UTC times               | RA<br>(deg) | Dec<br>(deg) | 50% err<br>(deg) | 90% err<br>(deg) | angular sep.<br>(deg) | time diff.<br>(s) | $\lambda$ | <i>Swift</i> XRT obs. |
|-----|---------------|-------------------------|-------------|--------------|------------------|------------------|-----------------------|-------------------|-----------|-----------------------|
| 228 | 56916.9606234 | 2014-09-16 23:03:17.858 | 32.74       | 75.12        | 0.2289           | 0.7887           | 3.36                  | 90.271275         | -0.373    |                       |
| 229 | 56918.2386039 | 2014-09-18 05:43:35.378 | 191.22      | 6.85         | 0.2318           | 0.7986           | 3.41                  | 94.220109         | 33.973    |                       |
| 230 | 56922.4369618 | 2014-09-22 10:29:13.497 | 75.05       | 2.25         | 0.6229           | 2.1474           | 2.82                  | 76.840695         | -5.595    |                       |
| 231 | 56927.7153963 | 2014-09-27 17:10:10.239 | 191.3       | 8.89         | 0.9266           | 3.1777           | 2.96                  | 12.422116         | -6.426    |                       |
| 232 | 56932.8573437 | 2014-10-02 20:34:34.498 | 135.48      | 3.16         | 0.5717           | 1.9778           | 2.69                  | 33.329884         | -7.736    |                       |
| 233 | 56937.2318703 | 2014-10-07 05:33:53.589 | 114.81      | 45.68        | 2.815            | 9.6914           | 3.43                  | 37.511792         | 1.123     |                       |
| 234 | 56939.1603754 | 2014-10-09 03:50:56.437 | 174.3       | 26.41        | 0.79             | 2.7129           | 2.62                  | 46.635442         | -6.011    |                       |
| 235 | 56940.1408902 | 2014-10-10 03:22:52.915 | 102.15      | 26.6         | 1.2139           | 4.1936           | 1.48                  | 28.056183         | -6.086    |                       |
| 236 | 56940.3352202 | 2014-10-10 08:02:43.029 | 253.38      | 21.02        | 0.4545           | 1.5738           | 2.82                  | 26.121765         | -8.292    |                       |
| 237 | 56947.1628326 | 2014-10-17 03:54:28.733 | 68.65       | 12.76        | 0.3768           | 1.3049           | 2.89                  | 79.649868         | -6.973    |                       |
| 238 | 56950.8863857 | 2014-10-20 21:16:23.727 | 103.75      | 4.28         | 1.1381           | 3.9715           | 2.37                  | 40.015829         | -5.114    |                       |
| 239 | 56952.6616545 | 2014-10-22 15:52:46.945 | 302.14      | 9.82         | 0.3457           | 1.1975           | 3.05                  | 47.692831         | -7.144    |                       |
| 240 | 56955.2166943 | 2014-10-25 05:12:02.389 | 8.01        | 9.03         | 0.6483           | 2.2461           | 2.32                  | 26.390761         | -8.291    |                       |
| 241 | 56963.9279414 | 2014-11-02 22:16:14.140 | 206.66      | 11.49        | 0.5138           | 1.7715           | 0.79                  | 56.164044         | -7.464    |                       |
| 242 | 56964.7877783 | 2014-11-03 18:54:24.041 | 41.62       | 37.04        | 1.3164           | 4.6369           | 1.83                  | 13.028268         | -5.682    |                       |
| 243 | 56966.8865966 | 2014-11-05 21:16:41.943 | 277.42      | 24.58        | 0.459            | 1.58             | 2.42                  | 27.627347         | -9.185    |                       |
| 244 | 56970.2139339 | 2014-11-09 05:08:03.888 | 34.79       | 28.52        | 0.9298           | 3.2017           | 3.35                  | 89.700106         | -3.193    |                       |
| 245 | 56970.2928569 | 2014-11-09 07:01:42.837 | 24.85       | 1.73         | 0.6495           | 2.2583           | 0.82                  | 10.226708         | -12.138   |                       |
| 246 | 56973.0685607 | 2014-11-12 01:38:43.647 | 272.12      | 11.29        | 1.3287           | 4.608            | 2.13                  | 7.226224          | -7.779    |                       |
| 247 | 56973.1423061 | 2014-11-12 03:24:55.246 | 274.17      | 36.54        | 0.8873           | 3.0523           | 3.01                  | 65.053504         | -3.6      |                       |
| 248 | 56979.2268092 | 2014-11-18 05:26:36.318 | 54.94       | 2.57         | 0.9725           | 3.3402           | 1.21                  | 48.861912         | -6.565    |                       |
| 249 | 56991.9067103 | 2014-11-30 21:45:39.767 | 255.06      | 22.45        | 0.7972           | 2.7407           | 2.51                  | 11.912897         | -9.031    |                       |
| 250 | 56992.1826576 | 2014-12-01 04:23:01.618 | 79.83       | 26.84        | 1.8199           | 6.2792           | 2.26                  | 47.29717          | -1.783    |                       |
| 251 | 57002.6178711 | 2014-12-11 14:49:44.060 | 63.07       | 32.74        | 0.3612           | 1.251            | 1.82                  | 80.407366         | -7.67     |                       |
| 252 | 57004.7245309 | 2014-12-13 17:23:19.466 | 128.65      | 2.05         | 0.6185           | 2.1292           | 2.61                  | 49.768765         | -6.204    |                       |
| 253 | 57007.6506045 | 2014-12-16 15:36:52.230 | 90.76       | 13.99        | 0.6425           | 2.2197           | 2.55                  | 84.822628         | -5.217    |                       |
| 254 | 57014.9337623 | 2014-12-23 22:24:37.062 | 52.37       | 33.67        | 1.3052           | 4.4889           | 2.86                  | 93.127713         | -2.158    |                       |
| 255 | 57015.2316342 | 2014-12-24 05:33:33.192 | 237.91      | 11.73        | 0.4836           | 1.6686           | 1.46                  | 38.224018         | -10.552   |                       |
| 256 | 57022.4814154 | 2014-12-31 11:33:14.287 | 311.67      | 6.07         | 0.5766           | 1.9881           | 3.28                  | 20.539414         | -4.734    |                       |
| 257 | 57024.5213094 | 2015-01-02 12:30:41.134 | 146.22      | 25.47        | 0.6868           | 2.3719           | 2.65                  | 97.344706         | -5.068    |                       |
| 258 | 57036.3894993 | 2015-01-14 09:20:52.736 | 39.31       | 5.83         | 0.7359           | 2.5352           | 2.05                  | 49.715639         | -7.261    |                       |
| 259 | 57037.3179683 | 2015-01-15 07:37:52.462 | 73.93       | 4.49         | 0.9407           | 3.2322           | 1.7                   | 68.1848           | -5.379    |                       |
| 260 | 57039.4466647 | 2015-01-17 10:43:11.828 | 353.22      | 9.47         | 0.3436           | 1.2032           | 2.98                  | 84.381224         | -6.987    |                       |
| 261 | 57045.5376424 | 2015-01-23 12:54:12.304 | 17.72       | 45.67        | 0.2083           | 0.7198           | 1.83                  | 27.874103         | -3.416    |                       |
| 262 | 57047.7086184 | 2015-01-25 17:00:24.627 | 19.96       | 2.66         | 0.5367           | 1.8571           | 2.08                  | 66.851165         | -7.211    |                       |
| 263 | 57052.3441571 | 2015-01-30 08:15:35.172 | 301.95      | 11.42        | 0.4621           | 1.5849           | 3.08                  | 24.270788         | -7.095    |                       |
| 264 | 57068.8696904 | 2015-02-15 20:52:21.252 | 284.77      | 45.43        | 0.2757           | 0.9546           | 3.07                  | 49.921954         | -8.362    |                       |
| 265 | 57071.5852633 | 2015-02-18 14:02:46.750 | 27.07       | 24.47        | 1.1232           | 3.8761           | 2.33                  | 4.505372          | -9.52     |                       |
| 266 | 57072.4809404 | 2015-02-19 11:32:33.254 | 135.75      | 1.85         | 0.4928           | 1.7035           | 2.87                  | 72.716739         | -3.668    |                       |
| 267 | 57074.252563  | 2015-02-21 06:03:41.440 | 288.01      | 2.43         | 0.5236           | 1.8027           | 3.12                  | 98.81793          | -5.153    |                       |
| 268 | 57078.6833597 | 2015-02-25 16:24:02.280 | 239.17      | 27.37        | 1.8058           | 6.1935           | 2.31                  | 60.214228         | -0.508    |                       |
| 269 | 57095.2011052 | 2015-03-14 04:49:35.485 | 284.87      | 11.78        | 0.4796           | 1.6557           | 0.46                  | 43.711471         | -12.162   | yes                   |
| 270 | 57103.248366  | 2015-03-22 05:57:38.818 | 51.68       | 49.26        | 0.7455           | 2.5806           | 0.28                  | 75.775181         | -4.882    |                       |
| 271 | 57104.2480613 | 2015-03-23 05:57:12.495 | 88.04       | 36.13        | 2.0106           | 6.9207           | 2.87                  | 32.100255         | -1.318    |                       |
| 272 | 57109.5669177 | 2015-03-28 13:36:21.687 | 65.76       | 19.89        | 0.7113           | 2.4609           | 2.23                  | 25.114433         | -8.271    |                       |
| 273 | 57109.7797106 | 2015-03-28 18:42:46.999 | 347.6       | 22.52        | 0.7362           | 2.5534           | 2.73                  | 99.686699         | -4.668    |                       |
| 274 | 57112.8077199 | 2015-03-31 19:23:06.996 | 233.88      | 7.83         | 0.2805           | 0.9738           | 3.41                  | 88.817669         | 0.166     |                       |
| 275 | 57116.6273979 | 2015-04-04 15:03:27.175 | 344.04      | 25.42        | 1.5215           | 5.3529           | 1.89                  | 83.473865         | -2.043    |                       |
| 276 | 57118.2715855 | 2015-04-06 06:31:04.985 | 334.66      | 13.55        | 0.326            | 1.1276           | 1.85                  | 9.629839          | -13.151   |                       |
| 277 | 57120.2643421 | 2015-04-08 06:20:39.159 | 153.66      | 26.72        | 0.8773           | 3.0249           | 3.16                  | 16.922026         | -7.063    |                       |
| 278 | 57130.3402053 | 2015-04-18 08:09:53.741 | 0.16        | 38.95        | 0.5768           | 1.9792           | 3.05                  | 29.689711         | -6.984    |                       |
| 279 | 57130.8076035 | 2015-04-18 19:22:56.943 | 122.34      | 9.97         | 0.649            | 2.2461           | 2.68                  | 73.305143         | -5.201    |                       |
| 280 | 57131.7993723 | 2015-04-19 19:11:05.765 | 167.87      | 69.75        | 1.0785           | 3.7016           | 2.78                  | 43.176918         | -4.826    |                       |
| 281 | 57138.7520932 | 2015-04-26 18:03:00.848 | 25.49       | 3.72         | 0.5726           | 2.018            | 1.76                  | 54.729134         | -8.277    |                       |
| 282 | 57161.6996759 | 2015-05-19 16:47:32.000 | 342.38      | 31.47        | 0.4416           | 1.5266           | 1.14                  | 11.999466         | -11.057   |                       |
| 283 | 57165.7059375 | 2015-05-23 16:56:33.000 | 137.61      | 32.21        | 0.6736           | 2.3232           | 3.14                  | 55.000359         | -5.622    |                       |
| 284 | 57173.521875  | 2015-05-31 12:31:30.000 | 116.28      | 1.25         | 0.3262           | 1.1188           | 2.87                  | 80.999919         | -7.371    |                       |
| 285 | 57173.6610995 | 2015-05-31 15:51:59.000 | 179.93      | 30.51        | 0.3994           | 1.3709           | 3.06                  | 33.999252         | -7.65     |                       |
| 286 | 57190.2258912 | 2015-06-17 05:25:17.000 | 7.13        | 4.6          | 0.4594           | 1.577            | 2.22                  | 65.999638         | -7.935    |                       |
| 287 | 57195.6324653 | 2015-06-22 15:10:45.000 | 286.69      | 12.26        | 0.8133           | 2.8124           | 2.57                  | 72.000144         | -5.196    |                       |
| 288 | 57205.3887153 | 2015-07-02 09:19:45.000 | 340.43      | 7.74         | 0.3154           | 1.0898           | 2.4                   | 89.000292         | -7.897    |                       |
| 289 | 57218.057581  | 2015-07-15 01:22:55.000 | 348.26      | 43.76        | 0.9262           | 3.1791           | 1.66                  | 14.99949          | -7.084    |                       |
| 290 | 57239.1376042 | 2015-08-05 03:18:09.000 | 324.78      | 4.76         | 0.6954           | 2.3938           | 3.31                  | 35.999735         | -5.289    |                       |
| 291 | 57239.6177315 | 2015-08-05 14:49:32.000 | 134.23      | 4.01         | 0.5075           | 1.747            | 3.06                  | 69.00031          | -2.564    |                       |
| 292 | 57251.348287  | 2015-08-17 08:21:32.000 | 168.94      | 2.73         | 0.7501           | 2.6029           | 1.8                   | 53.99966          | -7.436    |                       |
| 293 | 57260.8035417 | 2015-08-26 19:17:06.000 | 26.12       | 19.74        | 1.5              | 5.247            | 0.76                  | 60.999675         | -2.242    |                       |
| 294 | 57267.7290162 | 2015-09-02 17:29:47.000 | 181.79      | 21.39        | 0.5386           | 1.8646           | 0.88                  | 30.999774         | -10.855   |                       |
| 295 | 57281.5144907 | 2015-09-16 12:20:52.000 | 117.28      | 2.94         | 0.6501           | 2.2343           | 3.11                  | 83.000428         | -5.008    |                       |
| 296 | 57286.4959028 | 2015-09-21 11:54:06.000 | 308.37      | 15.28        | 0.6109           | 2.1036           | 3.03                  | 24.999738         | -7.693    |                       |
| 297 | 57305.0004861 | 2015-10-10 00:00:42.000 | 103.69      | 63.06        | 0.5767           | 1.9826           | 2.15                  | 5.00026           | -12.498   | yes                   |
| 298 | 57316.8767477 | 2015-10-21 21:02:31.000 | 280.47      | 3.32         | 0.4298           | 1.4762           | 2.12                  | 37.999863         | -7.581    |                       |
| 299 | 57335.8461458 | 2015-11-09 20:18:27.000 | 134.68      | 12.17        | 1.2074           | 4.1916           | 1.69                  | 93.99986          | -3.374    |                       |
| 300 | 57337.6787037 | 2015-11-11 16:17:20.000 | 280.31      | 10.47        | 1.187            | 4.0991           | 2.93                  | 37.000265         | -4.526    |                       |
| 301 | 57337.9006482 | 2015-11-11 21:36:56.000 | 156.44      | 7.97         | 1.186            | 4.1027           | 3.5                   | 95.999727         | -2.045    |                       |
| 302 | 57345.2203125 | 2015-11-19 05:17:15.000 | 300.02      | 3.77         | 0.3155           | 1.0925           | 0.57                  | 5.999962          | -18.006   | yes                   |
| 303 | 57349.9003935 | 2015-11-23 21:36:34.000 | 228.45      | 6.06         | 1.1676           | 4.2504           | 1.86                  | 68.000827         | -2.458    |                       |

TABLE 1 — *Continued*

| #                | MJD           | UTC times               | RA<br>(deg) | Dec<br>(deg) | 50% err<br>(deg) | 90% err<br>(deg) | angular sep.<br>(deg) | time diff.<br>(s) | $\lambda$ | <i>Swift</i> XRT obs. |
|------------------|---------------|-------------------------|-------------|--------------|------------------|------------------|-----------------------|-------------------|-----------|-----------------------|
| 304              | 57353.2239468 | 2015-11-27 05:22:29.000 | 238.47      | 11.29        | 0.5913           | 2.0422           | 2.97                  | 94.000117         | -3.577    |                       |
| 305              | 57354.0545602 | 2015-11-28 01:18:34.000 | 135.71      | 8.21         | 0.6668           | 2.308            | 3.41                  | 16.999775         | -6.208    |                       |
| 306              | 57375.8217477 | 2015-12-19 19:43:19.000 | 324.62      | 18.18        | 0.4248           | 1.4664           | 2.75                  | 97.000012         | -1.766    |                       |
| 307              | 57380.0829167 | 2015-12-24 01:59:24.000 | 116.71      | 38.5         | 0.716            | 2.4796           | 3.38                  | 22.000301         | -6.218    |                       |
| 308              | 57380.812338  | 2015-12-24 19:29:46.000 | 64.77       | 21.58        | 1.0836           | 3.7261           | 1.73                  | 6.000133          | -9.382    |                       |
| 309              | 57381.9145833 | 2015-12-25 21:57:00.000 | 61.3        | 36.57        | 0.8494           | 2.9188           | 2.54                  | 55.999977         | -5.643    |                       |
| 310              | 57385.6291782 | 2015-12-29 15:06:01.000 | 280.16      | 19.63        | 1.0185           | 3.4939           | 1.18                  | 39.999892         | -6.763    |                       |
| 311              | 57386.2039931 | 2015-12-30 04:53:45.000 | 323.05      | 7.76         | 0.2883           | 0.9939           | 3.35                  | 78.000346         | 18.992    |                       |
| 312              | 57387.6354398 | 2015-12-31 15:15:02.000 | 319.24      | 5.3          | 0.9237           | 3.1691           | 2.23                  | 31.999406         | -6.342    |                       |
| 313              | 57391.2709491 | 2016-01-04 06:30:10.000 | 145.44      | 6.2          | 0.6061           | 2.0989           | 2.4                   | 90.000564         | -4.659    |                       |
| 314              | 57395.7506597 | 2016-01-08 18:00:57.000 | 296.77      | 4.39         | 0.4324           | 1.5003           | 0.95                  | 56.000625         | -11.453   |                       |
| 315              | 57403.9758796 | 2016-01-16 23:25:16.000 | 334.44      | 16.55        | 0.2191           | 0.7587           | 2.59                  | 58.000329         | -8.67     |                       |
| 316              | 57411.9500926 | 2016-01-24 22:48:08.000 | 308.23      | 12.84        | 0.3116           | 1.0803           | 2.93                  | 90.999807         | -4.92     |                       |
| 317              | 57425.6187269 | 2016-02-07 14:50:58.000 | 355.56      | 6.77         | 0.6148           | 2.1215           | 2.38                  | 28.999982         | -8.17     |                       |
| 318              | 57429.0742593 | 2016-02-11 01:46:56.000 | 91.8        | 36.45        | 0.2304           | 0.7979           | 2.29                  | 19.999993         | -9.434    | yes                   |
| 319              | 57435.6070949 | 2016-02-17 14:34:13.000 | 206.65      | 3.28         | 0.8314           | 2.9181           | 3.19                  | 1.999608          | -11.049   |                       |
| 320 <sup>†</sup> | 57435.8066088 | 2016-02-17 19:21:31.000 | 24.62       | 38.01        | 1.071            | 3.681            | 2.48                  | 55.999367         | -3.722    | yes                   |
| 321 <sup>†</sup> | 57435.8066088 | 2016-02-17 19:21:31.000 | 27.14       | 40.62        | 0.964            | 3.3373           | 1.21                  | 87.00033          | -3.691    | yes                   |
| 322              | 57447.112882  | 2016-02-29 02:42:33.000 | 183.04      | 4.07         | 0.3192           | 1.1045           | 1.7                   | 49.999809         | -10.462   |                       |
| 323              | 57453.9627315 | 2016-03-06 23:06:20.000 | 200.84      | 4.07         | 0.4861           | 1.6692           | 1.81                  | 34.000408         | -9.536    |                       |
| 324              | 57455.9672222 | 2016-03-08 23:12:48.000 | 36.69       | 64.93        | 0.3746           | 1.4906           | 2.84                  | 29.9996           | -8.517    |                       |
| 325              | 57456.4267824 | 2016-03-09 10:14:34.000 | 316.67      | 7.9          | 0.894            | 3.0957           | 2.85                  | 59.000146         | -4.844    |                       |
| 326              | 57459.1598727 | 2016-03-12 03:50:13.000 | 231.12      | 13.85        | 0.7347           | 2.525            | 1.45                  | 85.000181         | -5.447    |                       |
| 327              | 57462.734213  | 2016-03-15 17:37:16.000 | 102.31      | 3.22         | 0.6906           | 2.3723           | 0.91                  | 13.999557         | -10.941   |                       |
| 328              | 57463.5895833 | 2016-03-16 14:09:00.000 | 182.85      | 39.49        | 0.3458           | 1.1903           | 1.5                   | 54.999659         | -10.408   |                       |
| 329              | 57468.7499769 | 2016-03-21 17:59:58.000 | 144.24      | 20.98        | 0.5894           | 2.0289           | 2.17                  | 8.999655          | -11.101   |                       |
| 330              | 57469.1791667 | 2016-03-22 04:18:00.000 | 265.25      | 68.1         | 0.5053           | 1.7399           | 0.34                  | 3.000278          | -17.272   |                       |
| 331              | 57475.0538773 | 2016-03-28 01:17:35.000 | 300.57      | 9.78         | 0.3481           | 1.2025           | 2.51                  | 48.000458         | -2.148    |                       |
| 332              | 57475.0776158 | 2016-03-28 01:51:46.000 | 252.6       | 22.72        | 0.6798           | 2.337            | 2.89                  | 0.999251          | -13.888   |                       |
| 333              | 57492.3056134 | 2016-04-14 07:20:05.000 | 8.71        | 24.37        | 0.4465           | 1.5463           | 3.34                  | 55.999875         | -5.952    |                       |
| 334              | 57496.3379398 | 2016-04-18 08:06:38.000 | 328.17      | 21.74        | 0.7019           | 2.4199           | 0.99                  | 84.999889         | -5.225    |                       |
| 335              | 57502.4096181 | 2016-04-24 09:49:51.000 | 303.24      | 3.13         | 0.5494           | 1.9076           | 2.27                  | 40.999886         | -7.658    |                       |
| 336              | 57508.8629745 | 2016-04-30 20:42:41.000 | 194.52      | 29.42        | 0.4773           | 1.7991           | 3.35                  | 37.000609         | -6.637    |                       |
| 337              | 57511.6773264 | 2016-05-03 16:15:21.000 | 189.69      | 21.78        | 0.4195           | 1.451            | 2.82                  | 36.000191         | -7.363    |                       |
| 338              | 57515.8865046 | 2016-05-07 21:16:34.000 | 317.69      | 47.13        | 0.7386           | 2.5611           | 2.54                  | 93.000048         | -4.929    |                       |
| 339              | 57515.9951042 | 2016-05-07 23:52:57.000 | 69.06       | 37.94        | 0.4715           | 1.6173           | 1.98                  | 61.999687         | -7.595    |                       |
| 340              | 57524.1083218 | 2016-05-16 02:35:59.000 | 247.53      | 20.53        | 2.3673           | 8.2044           | 2.31                  | 1.99965           | -5.931    |                       |

NOTE. — The MJD and UTC times refer to the detection time of the first neutrino. RA and Dec are the right ascension and declination of the weighted average direction. The 50% and 90% errors have been calculated by propagating the errors of the individual events. We further list the difference between the arrival times of the two events in seconds and their angular separation. The likelihood parameter  $\lambda$  is an estimate for the significance of the doublet where smaller values correspond to more significant and better localized alerts.  $\lambda$  has been calculated based on Equation 1 in Aartsen et al. (2015) using  $\theta = 0.5$  deg as the size of the field covered in tiled *Swift* XRT observations. The last column specifies whether *Swift* observations have been triggered.

<sup>†</sup> The doublets 321 and 322 have the first event in common and together from the triplet presented in Aartsen et al. (2016).
